# Supplementary material for: Analysis of Invariance and Robustness via Invertibility of ReLU-Networks
Source: arXiv:1806.09730 source file (2018-06-27)
Supplement: Supplementary file 1 [file appendix.pdf]

## A1 Appendix for Section 2

**Corollary 10** For  $A \in \mathbb{R}^{m \times n}$  the following statements are equivalent.

1.  $A$  is omnidirectional.
2.  $\nexists x \neq 0 : Ax \leq 0$
3.  $\nexists x \succeq 0 : Ax \leq 0$
4. Every linear open halfspace contains a row of  $A$ .
5.  $Ax \leq 0$  implies  $x = 0$ .

Here  $z \preceq 0$  means  $z \in \mathbb{R}_{\leq 0}^n$  and  $z \neq 0$ .

**Definition 11** (Convex hull)

For  $A \in \mathbb{R}^{m \times n}$ , the convex hull is defined as

$$\text{Conv}(A) = \left\{ \sum_{i=1}^m \alpha_i a_i : \forall i \alpha_i \in \mathbb{R}_{\geq 0} \wedge \sum_i \alpha_i = 1 \right\},$$

where  $a_i \in \mathbb{R}^n$  are the rows of  $A$ .

**Theorem 12** (Stiemke's theorem e.g. [9])

Let  $A \in \mathbb{R}^{m \times n}$  be a matrix, then the following two expressions are equivalent.

- $\nexists y : Ay \preceq 0$
- $\exists x > 0 : A^T x = 0$

Here  $z \preceq 0$  means that  $0 \neq z \leq 0$ .

**Theorem 13** (Singleton solutions of inequality systems)

Let  $A \in \mathbb{R}^{m \times n}$ ,  $b \in \mathbb{R}^m$  and  $x \in \mathbb{R}^n$ . Furthermore, let the inequality system

$$Ax + b \leq 0,$$

written as  $(A, b)$ , have a solution  $x_0$ .

Then this solution is unique if and only if there exists an index set,  $I$ , for the rows s.t.  $(A|_I, b|_I)$  is omnidirectional for  $x_0$ .

**Proof** (Theorem 13, Singleton solutions of inequality systems)

“ $\Leftarrow$ ”

Let  $(A|_I, b|_I)$  be omnidirectional for  $x_0$ . Then it holds that  $A|_I x + b|_I = A|_I (x - x_0) \leq 0$ . Due to the omnidirectionality of  $A|_I$ ,  $x_0$  is the unique solution of the inequality system  $A|_I x + b|_I \leq 0$ . The existence of a solution for the whole system  $Ax + b \leq 0$  is guaranteed by assumption and therefore  $x_0$  is the unique solution of  $Ax + b \leq 0$ .

“ $\Rightarrow$ ”

Here we will prove

$$\nexists I : (A|_I, b|_I) \text{ omnidirectional for some } p \Rightarrow \text{solution non-unique}.$$

We will start by doing the following logical transformations:

$$\begin{aligned} & \nexists I : (A|_I, b|_I) \text{ omnidirectional for some } p \\ \Leftrightarrow & \nexists (I, p) : (A|_I \text{ omnidirectional} \wedge b|_I = -A|_I p) \\ \Leftrightarrow & \forall (I, p) : \neg(A|_I \text{ omnidirectional} \wedge b|_I = -A|_I p) \\ \Leftrightarrow & \forall (I, p) : (A|_I \text{ not omnidirectional} \vee b|_I \neq -A|_I p). \end{aligned}$$

Now we define the vector  $c_0 := Ax_0 + b \leq 0$  and the set  $I$  as the index set given via  $c_0 = 0$ .

418 This means that  $A|_I$  is not omnidirectional, because otherwise  $A|_I x_0 + b|_I = 0$  due to the definition  
 419 of  $I$ , which would lead to the contradiction that  $(A|_I, b|_I)$  is omnidirectional for  $x_0$ . But this  
 420 means  $\exists x' \neq 0 : A|_I x' \leq 0$  as a result of Corollary 10. Since  $A|_{I^c} x_0 + b|_{I^c} < 0$ , we also have  
 421  $\forall x \exists \epsilon > 0 : A|_{I^c}(x_0 + \epsilon x) + b|_{I^c} < 0$ . This holds in particular for  $x'$ , so we define accordingly  
 422  $x^* := \epsilon x' \neq 0$ . Therefore, we have  $A|_{I^c}(x_0 + x^*) + b|_{I^c} < 0$  as well as

$$A|_I(x_0 + x^*) + b|_I = \underbrace{A|_I x_0 + b|_I}_{=c_0=0} + \underbrace{\epsilon A|_I x'}_{\leq 0} \leq 0.$$

423 Altogether it holds that  $A(x_0 + x^*) + b \leq 0$  with  $x^* \neq 0$ , which means that  $x_0$  is a non-unique  
 424 solution for the inequality system  $Ax + b \leq 0$ .  $\square$

425 **Proof** (Theorem 4, Preimages of ReLU-layers)

426 We consider the ReLU-layer

$$y = \text{ReLU}(Ax + b),$$

427 given its output  $y \in \mathbb{R}^m$  with  $A \in \mathbb{R}^{m \times n}$ ,  $b \in \mathbb{R}^m$  and  $x \in \mathbb{R}^n$ . Clearly, this equation can also be  
 428 written as the mixed linear system

$$\begin{aligned} A|_{y>0}x + b|_{y>0} &= y|_{y>0}, \\ A|_{y=0}x + b|_{y=0} &\leq 0. \end{aligned}$$

This allows us to consider the two cases

$$\mathcal{N}(A|_{y>0}) = \{0\} \text{ and } \mathcal{N}(A|_{y>0}) \neq \{0\}.$$

429 In the first case, we have a linear system which allows us to calculate  $x$  uniquely, i.e. we can do  
 430 retrieval. This leads us to the second case, the interesting one. In this case we can only recover  
 431  $x$  uniquely if and only if the system of inequalities “pins down”  $P_{\mathcal{N}(A|_{y>0})}x$ , where  $P_V$  is the  
 432 orthogonal projection into the closed space  $V$ . Formally this requires

$$A|_{y \leq 0}(P_{\mathcal{N}(A|_{y>0})^\perp}x + P_{\mathcal{N}(A|_{y>0})}x) + b|_{y \leq 0} \leq 0$$

433 to have a unique solution for  $x \in \mathbb{R}^n$  and  $P_{\mathcal{N}(A|_{y>0})^\perp}x$  fixed (given via the equality system). By  
 434 defining  $\bar{b} := b|_{y \leq 0} + A|_{y \leq 0}(P_{\mathcal{N}(A|_{y>0})^\perp}x)$  we have

$$A|_{y \leq 0}(P_{\mathcal{N}(A|_{y>0})}x) + \bar{b} \leq 0.$$

435 If  $O \in \mathbb{R}^{k \times n}$  now denotes an orthonormal basis of  $\mathcal{N}(A|_{y>0})$ , where  $k := \dim \mathcal{N}(A|_{y>0})$ , we can  
 436 write

$$\bar{A}\bar{x} + \bar{b} \leq 0,$$

437 where  $\bar{A} := AO^T$  and  $\bar{x} := Ox$  is a general element in  $\mathbb{R}^k$ . It now follows from Theorem 13 that  
 438 the inequality system  $(\bar{A}, \bar{b})$  has a unique solution if and only if  $(\bar{A}, \bar{b})$  has a subset of rows that are  
 439 omnidirectional for some point  $p$ .  $\square$

440 **Proof** (Theorem 5, Convex hull theorem)

441 Since  $\mathcal{N}(A) = \{0\}$  follows from both sides of the equivalence, the following sequence of equivalen-  
 442 cies holds.  $0 \in \text{Conv}(A)^\circ \Leftrightarrow \exists x > 0 : A^T x = 0 \xLeftrightarrow{\text{Theorem 12}} \nexists y : Ay \preceq 0 \xLeftrightarrow{\text{Corollary 10 and } \mathcal{N}(A) = \{0\}} \nexists y \neq 0 : Ay \leq 0$   
 443  $\nexists y \neq 0 : Ay \leq 0$   $\square$

## 444 A2 Proofs for section 3

445 **Proof** (Proof of Lemma 8, Global upper bound for largest/smallest singular value)

446 The upper bound on the largest singular value is trivial, as ReLU is contractive or in other terms  
 447  $\|D_I Ax\|_2 \leq \|Ax\|_2$  for all  $I$  and  $x \in \mathbb{R}^n$ .

448 To prove the upper bound for the smallest singular value, we assume

$$\sigma_M := \min\{\sigma_l : \sigma_l > 0\} > \tilde{\sigma}_k \tag{6}$$

449 and aim to produce a contradiction. Consider all singular vectors  $\tilde{v}_{k^*}$  with  $k^* \geq k$  from matrix  $A$ . It  
 450 holds for all  $\tilde{v}_{k^*}$

$$\tilde{\sigma}_k \geq \tilde{\sigma}_{k^*} = \|A\tilde{v}_{k^*}\|_2 \geq \|D_I A\tilde{v}_{k^*}\|_2, \tag{7}$$

451 as  $D_I$  is a projection matrix and thus only contracting. As

$$\sigma_M = \min_{\substack{\|x\|_2=1 \\ x \in \mathcal{N}(D_I A)^\perp}} \|D_I A x\|_2,$$

452 all  $\tilde{v}_{k^*} \notin \mathcal{N}(D_I A)^\perp$ . Otherwise, a  $\tilde{v}_{k^*}$  would be a minimizer by estimation (7), which would violate  
 453 the assumption (6).

454

455 Due to  $\mathcal{N}(D_I A)^\perp \oplus \mathcal{N}(D_I A) = \mathbb{R}^n$ , it holds  $\tilde{v}_{k^*} \in \mathcal{N}(D_I A)$ . As  $\tilde{v}_{k^*}$  are orthogonal,  
 456  $\dim(\text{span}(v_{k^*})) = |I| + 1$  (note:  $k^* = k, \dots, N$  and  $k = N - |I|$ , thus there are  $|I| + 1$  singular  
 457 vectors  $v_{k^*}$  in total). Furthermore,  $\tilde{v}_{k^*}$  were not in  $\mathcal{N}(A)$  by definition (corresponding singular  
 458 values were strictly positive).

459 Hence, the nullspace of  $D_I$  must have  $\dim(\mathcal{N}(D_I)) \geq |I| + 1$ . But  $D_I$  is the identity matrix except  
 460  $|I|$  zeros on the diagonal, thus  $\dim(\mathcal{N}(D_I)) = |I|$ , which yields a contradiction.  $\square$

461 **Proof** (Proof of Lemma 9, Weakly correlated rows)

462 Consider  $v = \frac{a_k}{\|a_k\|_2}$ . Then,

$$(D_I A v)_k = 0,$$

463 since  $k \in I$  ( $k$ -th row of  $D_I$  is zero). Furthermore, for all  $j \neq k$  it holds by condition (4)

$$(D_I A v)_j = \frac{\langle a_k, a_j \rangle}{\|a_k\|_2} \leq \frac{|\langle a_k, a_j \rangle|}{\|a_k\|_2} \leq \frac{c}{\sqrt{M}}.$$

464 Hence,

$$\|D_I A v\|_2 = \sqrt{\sum_{j \notin I} \left( \frac{\langle a_k, a_j \rangle}{\|a_k\|_2} \right)^2} \leq \sqrt{M \left( \frac{c}{\sqrt{M}} \right)^2} = c.$$

465 As  $a_k \in \mathcal{N}(D_I A)^\perp$ ,  $v \in \mathcal{N}(D_I A)^\perp$  as well. Thus,

$$\sigma_K = \min_{\substack{\|x\|_2 \\ x \in \mathcal{N}(D_I A)^\perp}} \|D_I A x\|_2 \leq \|D_I A v\|_2 \leq c.$$

466

$\square$

## 467 A3 Appendix for Section 2.2

In this section, we formulate the algorithm to determine whether the preimage of  $y$  given by

$$y = \text{ReLU}(Ax + b)$$

468 is finite.

469 This requires to check whether  $\bar{A}$  (see Theorem 4) is omnidirectional, which is equivalent to

$$0 \in \text{Conv}(\bar{A})^\circ,$$

470 see Theorem 5. Since it is reasonable to assume that 0 will not lie on the boundary of the convex  
 471 hull, we can formulate this as a *linear programming* problem. The side-conditions incorporate the  
 472 definition of convex hulls (Definition 11, Appendix A1). The objective function is chosen arbitrary,  
 473 as we are only interested in a solution.

---

### Algorithm 1 Finite preimage

---

**Input:**  $A \in \mathbb{R}^{m \times n}$ ,  $b \in \mathbb{R}^m$ ,  $y \in \mathbb{R}^m$   
**if**  $\text{rank}(A|_{y>0}) = n$  **then**  
     **return** True {Preimage is a singleton}  
**end if**  
 $O \leftarrow$  orthonormal basis of  $\mathcal{N}(A|_{y>0})$ , ( $\in \mathbb{R}^{k \times n}$ )  
 $\bar{A} \leftarrow A|_{y=0} O^T$ , ( $\in \mathbb{R}^{\tilde{k} \times k}$ )  
**if**  $\tilde{k} \leq k$  **then**  
     **return** False {see Corollary 6}  
**end if**  
 $c \leftarrow (1; \dots; 1)$  {arbitrary objective}  
  
**return** Does a solution for the linear program  $\left\{ \begin{array}{l} \max c^T x \\ \text{subject to} \\ \bar{A}^T x = 0 \\ (1; \dots; 1)^T x = 1 \\ x \in [0, 1]^{\tilde{k}} \end{array} \right.$  exists?

---

## 474 A4 Architectures for Numerical Studies

475 Training details for MLP on MNIST:

- 476 • Training using Adam optimizer [16]
- 477 • Epochs: 25
- 478 • Batch size: 1000

479 Training details for WideCIFAR and ThinCIFAR:

- 480 • Training setup from Keras [5] examples: cifar10\_cnn
- 481 • No data augmentation
- 482 • RMSprop optimizer
- 483 • Epochs: 100
- 484 • Batch size: 32

Table 1: Architecture of MLP trained on MNIST

| Index | Type                  | kernel size | stride | # feature maps | # output units |
|-------|-----------------------|-------------|--------|----------------|----------------|
| 0     | Input layer           | -           | -      | 3              |                |
| 1     | Dense layer           | -           | -      | -              | 100            |
| 2     | Dense layer           | -           | -      | -              | 100            |
| 3     | Dense layer           | -           | -      | -              | 100            |
| 4     | Dense layer           | -           | -      | -              | 100            |
| 5     | Dense layer           | -           | -      | -              | 100            |
| 6     | Dense layer           | -           | -      | -              | 100            |
| 7     | Dense layer           | -           | -      | -              | 100            |
| 8     | Dense layer           | -           | -      | -              | 100            |
| 9     | Dense layer           | -           | -      | -              | 100            |
| 10    | Dense layer           | -           | -      | -              | 100            |
| 11    | Dense layer (softmax) | -           | -      | -              | 10             |

Table 2: Architecture of MLP trained on MNIST

| Index | Type                  | kernel size | stride | # feature maps | # output units |
|-------|-----------------------|-------------|--------|----------------|----------------|
| 0     | Input layer           | -           | -      | 3              |                |
| 1     | Dense layer           | -           | -      | -              | 3500           |
| 2     | Dense layer           | -           | -      | -              | 784            |
| 3     | Dense layer (softmax) | -           | -      | -              | 10             |

Table 3: Architecture of WideCIFAR

| Index | Type                  | kernel size | stride | # feature maps | # output units |
|-------|-----------------------|-------------|--------|----------------|----------------|
| 0     | Input layer           | -           | -      | 3              |                |
| 1     | Convolutional layer   | (3,3)       | (1,1)  | 32             | -              |
| 2     | Convolutional layer   | (3,3)       | (2,2)  | 64             | -              |
| 3     | Convolutional layer   | (3,3)       | (1,1)  | 64             | -              |
| 4     | Convolutional layer   | (3,3)       | (1,1)  | 32             | -              |
| 5     | Convolutional layer   | (3,3)       | (1,1)  | 32             | -              |
| 6     | Convolutional layer   | (3,3)       | (2,2)  | 64             | -              |
| 7     | Dense layer           | -           | -      | -              | 512            |
| 8     | Dense layer (softmax) | -           | -      | -              | 10             |

Table 4: Architecture of ThinCIFAR

| Index | Type                  | kernel size | stride | # feature maps | # output units |
|-------|-----------------------|-------------|--------|----------------|----------------|
| 0     | Input layer           | -           | -      | 3              |                |
| 1     | Convolutional layer   | (3,3)       | (1,1)  | 32             | -              |
| 2     | Convolutional layer   | (3,3)       | (2,2)  | 32             | -              |
| 3     | Convolutional layer   | (3,3)       | (1,1)  | 16             | -              |
| 4     | Convolutional layer   | (3,3)       | (1,1)  | 16             | -              |
| 5     | Convolutional layer   | (3,3)       | (1,1)  | 16             | -              |
| 6     | Convolutional layer   | (3,3)       | (2,2)  | 32             | -              |
| 7     | Dense layer           | -           | -      | -              | 512            |
| 8     | Dense layer (softmax) | -           | -      | -              | 10             |

## A5 Numerical Analysis of Lemma 9

In order to better understand the bound on the smallest singular value after ReLU, given by Lemma 9, we numerically proceed as follows:

1. We choose  $c \in [a, b]$ , where  $a, b$  are suitable interval endpoints.

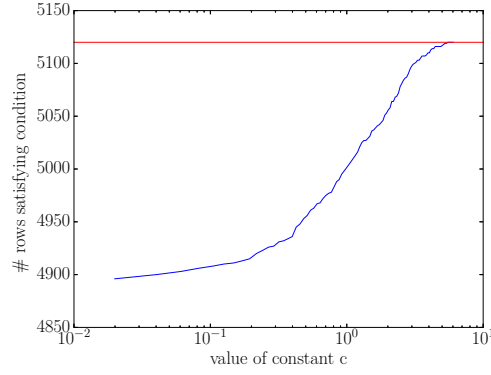

Figure 8: Curve showing how many rows  $a_i$  satisfy condition (4) from Lemma 9 depending on values of constant  $c$ . The red line shows the total number of remaining rows after removal by ReLU,  $M = 5120$ . Even for small constants  $c$  most  $a_i$  fulfill condition (4), yet not all, which is required by the lemma to give an upper bound on the smallest singular value. The example is from layer 4 of WideCIFAR, for only one sample from the test set.

- 489        2. Given  $c$ , we compute for every  $a_k$  with  $k \in I$  the value of  $c \frac{\|a_k\|_2}{\sqrt{M}}$  ( $M$  is the number of  
490            remaining rows, in the example  $M = 5120$ ).
- 491        3. For every  $a_k$  we count the number of  $a_i$  satisfying

$$|\langle a_i, a_k \rangle| \leq c \frac{\|a_k\|_2}{\sqrt{M}}.$$

- 492        4. We take the  $a_k$  with the maximal number of  $a_i$  satisfying the condition. (Note, that this  
493            ignores the requirement  $a_k \in \mathcal{N}(D_I A)^\perp$ .)
- 494        5. If we have an  $a_k$ , where all  $a_i$  satisfy the condition, the corresponding constant  $c$  gives the  
495            upper bound on the smallest singular value after ReLU.

496        Figure 8 shows the number of  $a_i$  satisfying the correlation condition given different choices of  $c$ . The  
497        red line is reached for  $c \approx 6$ . However, even the largest singular value after ReLU is smaller than  
498        2.5 (shown in Figure 5). Thus, the bound given by Lemma 9 is far off. This can be explained by the  
499        fact, that this situation is quite redundant ( $M = 5120$ ) and there are rows  $a_i$  still correlated to the  
500        removed rows  $a_k$ .

501        However, in the further Experiments on ThinCIFAR, we observe (see Figure A6) a stronger effect of  
502        ReLU in layer 2, which can be explained by having a less redundant scenario with fewer remaining  
503        rows.

## 504 A6 Further Experiments

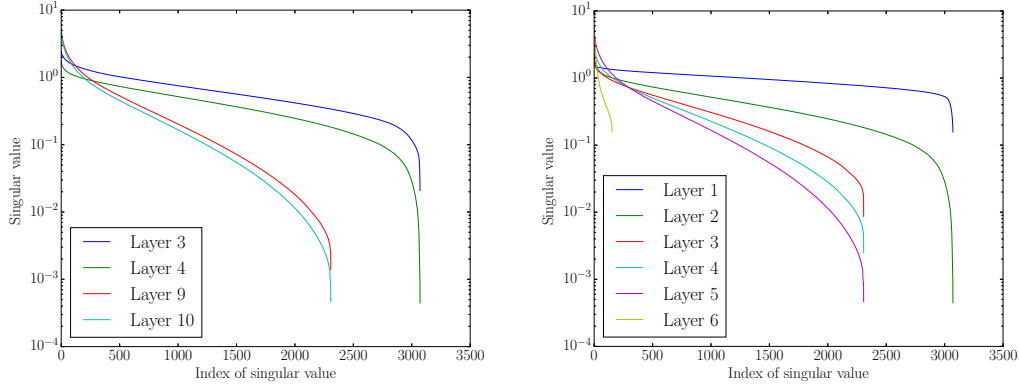

Figure 9: Left: Effect of ReLU on the singular values for ThinCifar. The curves show the effect in layer 2 (layer 3 and 4 in legend, because ReLU is counted as an extra activation layer) and layer 5 (layer 9 and 10). Right: Decay of singular values over the layers ThinCifar. Here, each layer includes the convolution and ReLU-activation. Reported number are taken from median over 50 samples. Best viewed in color.

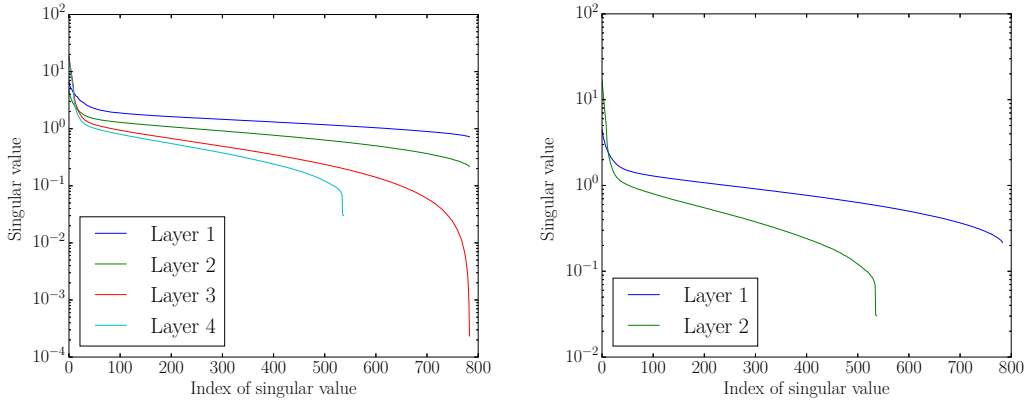

Figure 10: Left: Effect of ReLU on the singular values for the MLP on MNIST. The curves show the effect in layer 1 (layer 1 and 2 in legend, because ReLU is counted as an extra activation layer) and layer 2 (layer 3 and 4). Right: Decay of singular values over the layers of MLP on MNIST. Here, each layer includes the fully-connected layer and ReLU-activation. Reported number are taken from median over 50 samples.

## 505 A7 Invariance Experiment using an MLP on MNIST

506 This section briefly describes how the results in Figure 1 from the introduction were obtained (copied  
 507 in Figure 11 for readability). After training the network from 1 (in Appendix A4), we searched the  
 508 MNIST test set for input images with yielded the fewest positive activations in the first layer, in  
 509 the figure the digits "3" and "4". After selecting the example input  $x^*$ , we selected another input  $c$   
 510 belonging to a different class (e.g. a "6" and "4" in the first example).

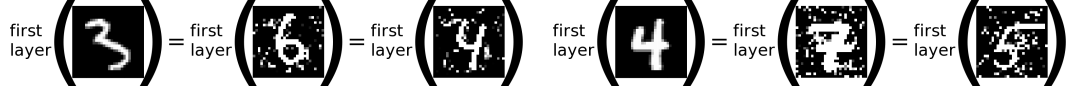

Figure 11: Invariances of the first layer (100 ReLU neurons) of a vanilla MLP. (Exact architecture in Appendix A4 Table 1.)

511 Afterwards, we solved following linear programming problem to find a perturbed  $x$ :

$$\begin{cases} \max \langle c, x \rangle \\ \text{subject to} \\ A|_{y^* > 0} x + b|_{y^* > 0} = y^*|_{y^* > 0} \quad , \\ A|_{y^* < 0} x + b|_{y^* < 0} \leq 0 \\ x \in [0, 1]^{\tilde{k}} \end{cases}$$

512 where the features of the first layer are computed via

$$y^* = \text{ReLU}(Ax^* + b).$$

513 Hence, we searched within the preimage of the features  $y^*$  of the first layer for examples  $x$  which  
 514 resemble images  $c$  from another class. By doing this we observe, that the preimages of the MLP may  
 515 have large volume. In these cases, the network is invariant to some semantics changes which shows  
 516 how the study of preimages can reveal previously unknown properties.

517
